# Supplementary material for: An integrated lithium-niobate electro-optic platform for spectrally tailored dual-comb spectroscopy
Source: arXiv:2003.04533 ancillary file (2020-03-11)
Supplement: Supplementary file 1 [file Arxiv___Dual_EO_COMB__SUPP.pdf]

# Supplemantary Information for: An integrated lithium-niobate electro-optic platform for spectrally tailored dual-comb spectroscopy

Amirhassan Shams-Ansari,[1,*] Mengjie Yu,[1,*] Zaijun Chen,[2,*] Christian Reimer,[1,3] Mian Zhang,[1,3] Nathalie Picqué,[2,†] and Marko Lončar[1,‡]

[1] *John A. Paulson School of Engineering and Applied Sciences, Harvard University, Cambridge, Massachusetts 02138, USA*

[2] *Max-Planck-Institut für Quantenoptik, Hans-Kopfermann-Str. 1, 85748 Garching, Germany*

[3] *HyperLight Corporation, 501 Massachusetts Ave, Cambridge, MA 02139, USA*

(Dated: March 10, 2020)

## I. DEVICE FABRICATION AND CHARACTERIZATION

The electro-optic (EO) racetrack microresonators are fabricated on a commercial 600 nm-thick X-cut lithium niobate (LN) wafer on 2-$\mu$m thermally grown silicon dioxide on a 500-$\mu$m silicon handle substrate (NanoLN). The waveguides and racetracks are defined using negative-tone resist (Fox16–Dow Corning) and electron-beam lithography (Elionix-F125) through multipass exposure. The pattern is then transferred to LN with a standard $Ar^{+}$ reactive ion etching [1]. The targeted etch depth for our devices is 350 nm leaving around 250 nm of LN slab underneath. The devices are then cladded with 1-$\mu$m thick silicon dioxide, deposited using plasma-enhanced chemical vapor deposition. A second photolithography (Heidelberg-MLA150) is performed (positive tone SPR-700 photoresist) to pattern the electrodes with 8 $\mu$m separation. Layers of a thickness of 15 nm of Ti and 500 nm of Au are deposited using electron-beam evaporation (Denton) as the metallic contacts. Finally, after a lift-off process, the chips are diced, and their facets are mechanically polished for lensed-fiber coupling. The straight sections of the racetrack cavity ( 6mm) and the gold microwave electrodes are patterned along the y-axis of the LN crystal resulting in the electric-field along the z-direction. This ensures that LN's highest EO tensor component is utilized. We select a ground-signal-ground (GSG) configuration for the microwave electrodes in order to simultaneously modulate the light travelling in each arm of the optical cavity (Fig. S1). The optical insertion loss of each device is evaluated to be 7 dB/facet. To suppress the input signal, a drop-port is fabricated, using the same waveguide-to-resonator gap (650 nm) as in the case of the through port. The full-width at half maximum of the cavity resonance, estimated from the Lorentzian fit, is 158 MHz ( 1.4 pm) corresponding to a loaded quality factor of about 106. The quality factor is mainly limited by the presence of the drop-port which introduces another loss channel for the photons inside the cavity (Fig. S2). For the free spectral range of 10.45 GHz, the cavity finesse, and the equivalent number of round-trips of the light inside the cavity (i.e. finesse/$2\pi$) are calculated to be 66 and 10, respectively.

## II. DEVICE OPERATION

In our experiment, the microresonator is optically injected with a CW-laser at a transverse-electric (TE) polarization, and it is driven by a microwave signal, provided by an amplified microwave-frequency synthesizer. The cavity resonances are identified by monitoring the transmission through the through-port while sweeping the input laser frequency. Next, the microwave signal is turned on to identify the cavity mode with the highest EO response - as manifested by a large resonance-broadening [1, 2]. The microwave frequency is then finely tuned to match the free spectral range of the cavity. The laser is tuned into the cavity resonance till the broadest possible EO-Comb spectrum is generated. With microwave and optical sources tuned into resonance, the output fiber is aligned to the drop port and the optical signal is collected. The drop-port device allows for suppression of the carrier and thus adapts the dynamic range of the dual-comb interferometer to the optical signal of interest.

## III. DETAILED DESCRIPTION OF THE DUAL-COMB SET-UP

We first describe the configuration (Fig.S3) using a single CW laser, used for producing the spectra shown in Figures 2 and 3. The entire set-up is realized with single-mode optical fibers. The beam of a single-frequency CW laser, of frequency $f_1$ in the telecommunication region, is split into two beams. The frequency of one of the beams is shifted to $f_1+\delta f_1$ with an acousto-optic frequency shifter (AOFS). In our set-up, $\delta f_1$=40 MHz. The role of the AOFS is to shift the center of the RF dual-comb spectrum to $\delta f_1$. If this were not performed, the optical carrier $f_1$ would be mapped at the zero frequency in the dual-comb spectroum and the pair of comb lines of index -n on one side of the optical carrier would be aliased at the same RF frequency as the pair of the comb lines of index n on the other side of the carrier. The use of an AOFS to avoid aliasing is already commonly reported in dual-comb spectroscopy experiments with bulk EO modulators [3, 4]. The optical beams are coupled in and out their corresponding chips, with racetrack resonators labeled EO-Comb source1 and EO-Comb source2, using lensed fibers. Two separate LN chips are used, one of which is equipped with a thermoelectric cooler. Frequency-tuning of the laser enables to match the laser frequency and one resonance of EO-Comb source1. For overlapping the resonance of EO-Comb source2 and the laser line, adjustment of the second chip temperature is used, with the thermoelectric cooler. Each cavity is modulated at a microwave frequency which matches, or is close to, the free spectral range of the cavity. The microwave signal is provided by a commercial synthesizer and is delivered to gold electrodes placed on each side of the waveguides in the ring using RF probes. One of the microwave synthesizers driving the chip is phase-locked to the internal 10-MHz clock of the other. For EO-Comb source1, the radio-frequency is $f_{RF1}$=10.45 GHz and for EO-Comb source2, it is varied such that $f_{RF2}$-$f_{RF1}$ ranges from 0.001 MHz to 0.8 MHz. An absorbing sample, at room temperature (293 K), consisting of a fiber-coupled multipass gas cell filled with acetylene (80-cm path length, $9.86\times10^{4}$-Pa pressure

of acetylene in natural abundance) may be placed on the beam path of EO-Comb source1. A manual polarization controller, also on the beam path of EO-Comb source1, adjusts the relative polarization of the two beams to maximize the interference signal. The beams from EO-Comb source1 and EO-Comb source2 are then combined onto a 50:50 fiber coupler. The two outputs of the coupler are detected by a balanced photodetector with a frequency bandwidth of 150 MHz. The output of the balanced photodetector is electronically filtered to about 50 MHz and amplified. The resulting time-domain interference signal is digitized using a 16-bit data acquisition board with a rate of $125\times10^6$ samples/s. The interferograms are Fourier transformed per segments of $5\times10^{-3}$ seconds, corresponding to 625000 time-domain samples. The duration of $5\times10^{-3}$ seconds is selected as it is experimentally determined to correspond to the time for which one can compute the spectrum without visible distortion to the instrumental line-shape (mutual coherence time). Before the complex transform is calculated, the interferograms are zero-filled six-fold to interpolate the spectra. The amplitude (absorption spectrum) and the phase (dispersion spectrum) are then averaged 19000-fold up to a total measurement time of 95 seconds. The RF spectrum is composed of lines at $\delta f_1+n(f_{RF2}\text{-}f_{RF1})$, where n is an integer. The computation procedure is validated by the perfect instrumental line-shape, obtained before and after the averaging process (Fig.2b), and by the square-root evolution of the signal-to-noise ratio of the comb lines as a function of the averaging time (Fig.2c). Each comb line appears as a cardinal sine, which is the instrumental line-shape of the spectrometer (Fig.2b). The interferogram is indeed multiplied by a boxcar function, which corresponds to the finite measurement time. Therefore, in the spectral domain, the comb lines are convolved by a cardinal sine which has a width equal to 1.2 times the inverse of the measurement time. In Fig. 2b, the full-width at half-maximum of the comb line is 240 Hz. This is 1.2 times the inverse of the measurement time of $5\times10^{-3}$ s, used in the computation of each interferogram. Our observed line width exactly corresponds to the transform-limited expected value for the transform of time-domain traces of $5\times10^{-3}$ s. The optical scale can be reconstituted a posteriori by substituting $\delta f_1$ for $f_1$ and $f_{RF2}$-$f_{RF1}$ for $f_{RF1}$. When spectral tailoring is implemented, as in the set-up sketched in Figure 4, several (two in Fig. 4) CW lasers are simultaneously injected in the two EO microrings. The two CW lasers in Fig. 4 emit at the optical frequencies $f_1$ and $f_2$, respectively. Each laser beam is split into two beams, one of which is sent into an AOFS driven at a frequency of $\delta f_1$ and $\delta f_2$, respectively. In our experiment $\delta f_1$=40 MHz and $\delta f_2$= 25 MHz. We used two RF shifts $\delta f_1$ and $\delta f_1$ rather distant because of the availability of the equipment. In practice it would be possible to interleave the two RF spectra provided that $\delta f_2$ is different from $\delta f_1$. The laser beams at frequencies $f_1$ and $f_2$ are combined and sent into EO-Comb source1, while the beams at shifted frequencies $f_1+\delta f_1$ and $f_2+\delta f_2$ are combined and sent into EO-Comb source2. At the output of the microring EO-Comb source1, two comb spectra, centered at frequencies $f_1$ and $f_2$ are produced. In the example of Fig.S4, the two spectra, measured with a commercial optical spectrum analyzer, are separated by 6.6 THz. Similar spectra are obtained for EO-Comb source2. When the signals of EO-Comb source1 and EO-Comb source2 beat on the fast photo-detector, the dual-comb spectrum (of a free spectral range of $f_1/2$) contains two RF combs, one centered at $\delta f_1$ and the other centered at $\delta f_2$. They both have a line spacing of ($f_{RF2}$-$f_{RF1}$), and they are not expected to be mutually coherent. The comb centered at $\delta f_1$ reports on the absorption and dispersion experienced by the sample in the region of the optical frequency $f_1$, while the comb centered at $\delta f_2$ corresponds to optical frequencies around $f_2$. The optical frequencies $f_1$ and $f_2$ can be adjusted independently.

## IV. COMPUTATION OF REFERENCE SPECTRA USING LITERATURE DATA

The acetylene computed transmittance spectrum (Fig. 3a) is calculated using the simulation tool on "HITRAN on the web"[5], that takes its line parameters from the HITRAN database [6]. Lorentzian line profiles are chosen. The computed dispersion spectrum (Fig. 3b) is derived from the calculated transmittance spectrum using the Kramers–Kronig relations [7].

---

* These authors contributed equally to this work
† nathalie.picque@mpq.mpg.de
‡ loncar@seas.harvard.edu

[1] M. Zhang, C. Wang, R. Cheng, A. Shams-Ansari, and M. Lončar, "Monolithic ultra-high-q lithium niobate microring resonator," *Optica*, vol. 4, no. 12, pp. 1536–1537, 2017.

[2] C. Reimer, Y. Hu, A. Shams-Ansari, M. Zhang, and M. Loncar, "High-dimensional frequency crystals and quantum walks in electro-optic microcombs," *arXiv preprint arXiv:1909.01303*, 2019.

[3] D. A. Long, A. J. Fleisher, K. O. Douglass, S. E. Maxwell, K. Bielska, J. T. Hodges, and D. F. Plusquellic, "Multiheterodyne spectroscopy with optical frequency combs generated from a continuous-wave laser," *Optics letters*, vol. 39, no. 9, pp. 2688–2690, 2014.

[4] G. Millot, S. Pitois, M. Yan, T. Hovhannisyan, A. Bendahmane, T. W. Hänsch, and N. Picqué, "Frequency-agile dual-comb spectroscopy," *Nature Photonics*, vol. 10, no. 1, pp. 27–30, 2016.

[5] http://hitran.iao.ru.

[6] I. E. Gordon, L. S. Rothman, C. Hill, R. V. Kochanov, Y. Tan, P. F. Bernath, M. Birk, V. Boudon, A. Campargue, K. Chance, *et al.*, "The hitran2016 molecular spectroscopic database," *Journal of Quantitative Spectroscopy and Radiative Transfer*, vol. 203, pp. 3–69, 2017.

[7] M. Sheik-Bahae, "Nonlinear optics basics. kramers-kronig relations in nonlinear optics," *Encyclopedia of modern optics*, pp. 234–239, 2005.

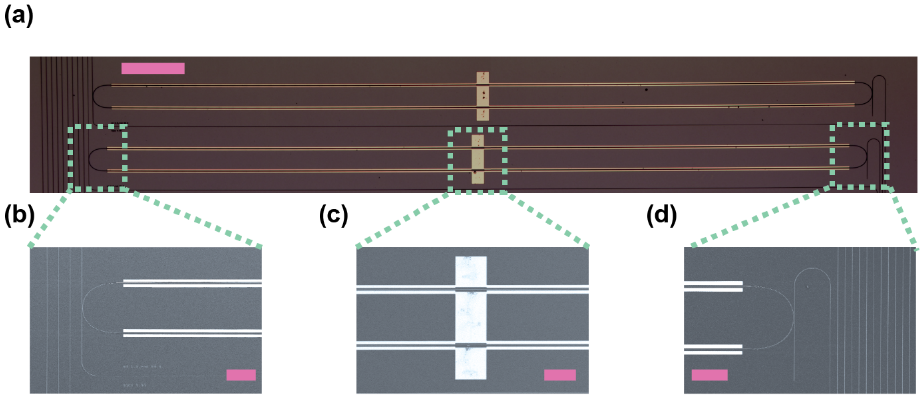


FIG. 1. **(a)** Microscope image of two fabricated lithium-niobate microresonators (the purple scale-bar represents 500$\nu$m). **(b)** Scanning electro-micrograph (SEM) of the coupling region (scale-bar represents 100 $\nu$m) **(c)** SEM of the microwave-probe metallic pad (scale-bar represents 100 $\nu$m)**(d)** SEM of the drop-port (scale-bar represents 100 $\nu$m).

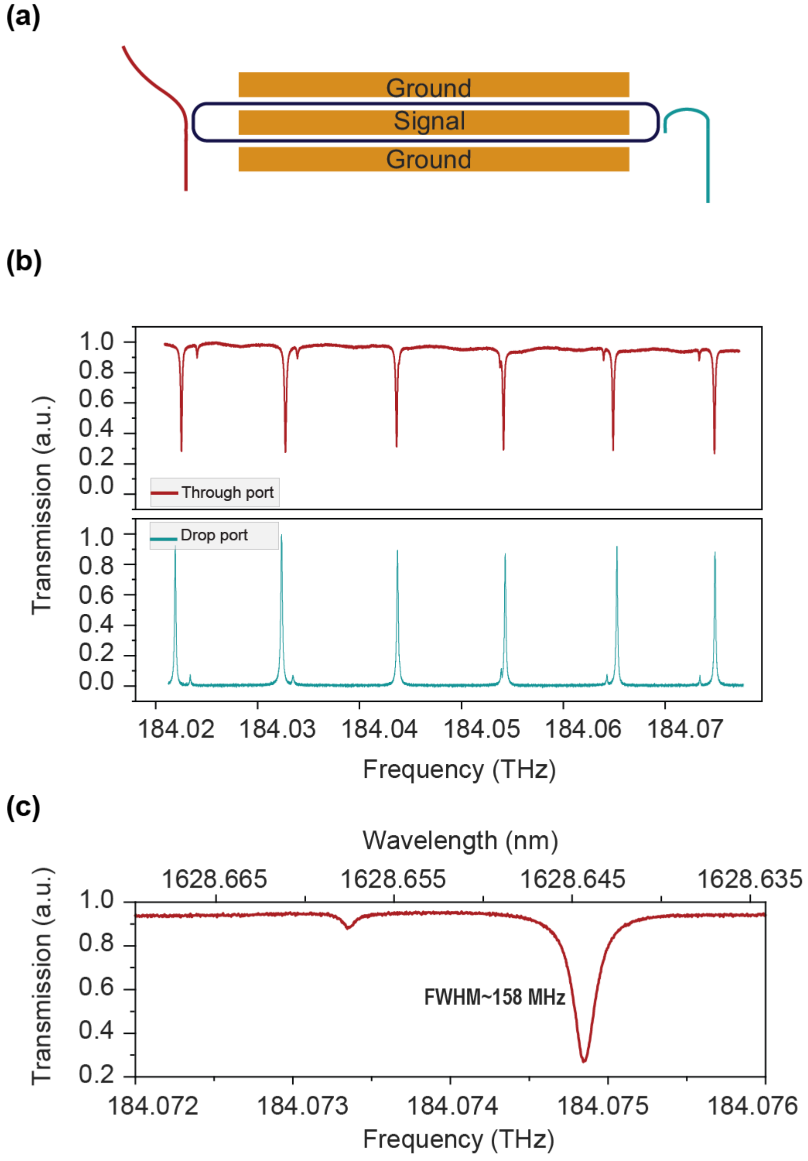


FIG. 2. **(a)** MA schematic EO-Comb source device with a drop-port. **(b)** The normalized transmission spectrum of the device detected by the photodiode from the through port (red) and the drop port (green) with a free spectral range of 10.45 GHz **(c)**The resonance of the ring with the full width at half maximum (FWHM) of 158 MHz ( 1.4 pm) corresponding to a Q-factor of $1.16\times10^6$.

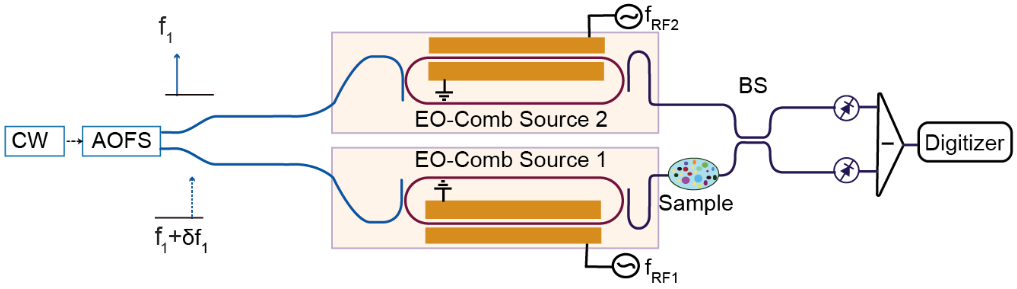


FIG. 3. **(a)** Experimental setup for dual-comb spectroscopy for the acetylene gas cell at near atmospheric pressure with two EO-Comb sources (CW: Continuous-wave laser, AOFS: Acousto-optic frequency shifter; BS: Beam splitter).

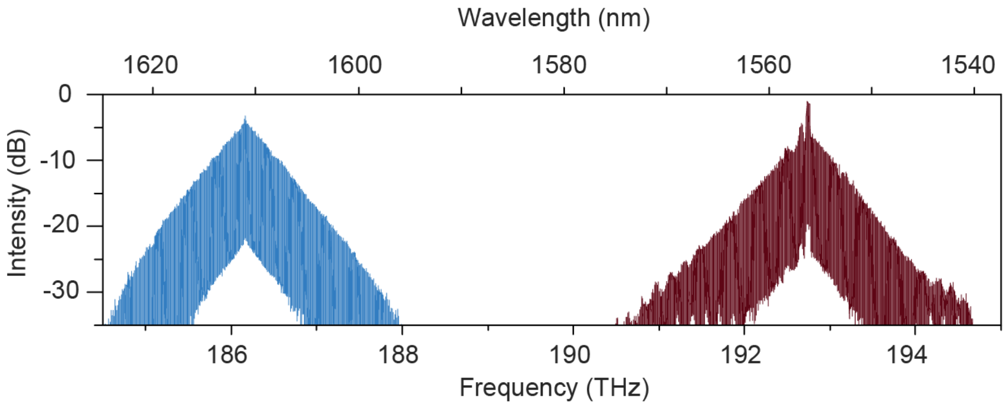


FIG. 4. The optical spectrum of a single EO-Comb source generator fed by two CW lasers. The spectrum consists of two frequency comb spectra separated by 6.6 THz in the telecommunication region. The spectrum is measured with an optical spectrum analyzer.
